# Supplementary material for: Implications of Regulations on the Use of AI and Generative AI for Human-Centered Responsible Artificial Intelligence
Source: arXiv:2403.00148 source file (2024-02-29)
Supplement: Supplementary file 1 [file appendix.tex]

\clearpage
\thispagestyle{empty}

\section*{Supplementary Material for Implications of AI Regulations and Generative AI for Human-Centered Responsible Artificial Intelligence}

\subsection*{Target Community \& Attendees}
We anticipate that participants will have expertise in either Human-Computer Interaction (HCI) or Artificial Intelligence (AI), and share a keen interest in the ethical aspects of AI. Participants are expected to contribute insights from both AI's technical aspects and HCI's social and human dimensions. Facilitating dialogue and exchange between these two groups is a central objective of this SIG. Attendees from both academic and industrial circles are expected, aiming to bridge the often so-called ``gap between academia and industry.'' We will also encourage participants from all career stages (e.g., from students and early career researchers to senior distinguished researchers) to join the SIG.

To promote the SIG, we plan to advertize it through various social media platforms, including Mastodon, Twitter, LinkedIn, and Facebook CHI Meta. Additionally, our network will be instrumental in drawing more participants, as the authors have relevant experience in these areas. Leveraging the diverse organizing team's network, we foresee to attract a diverse range of attendees, from students newly interested in the field to senior professionals with extensive experience.

\subsection*{Presentation \& Schedule}
We will use Miro, an online collaboration tool, to facilitate the discussion in the SIG. Below, we propose our schedule:

\begin{itemize}
    \item Introduction (10 minutes): The organizers will briefly introduce themselves and the SIG. Depending on the number of attendees, we may have a quick round-table session for short introductions.
    \item Group activity (20 minutes): Attendees will be divided into groups of 4-8 (depending on the number of attendees) to work on a Miro board. In this session, they will discuss current trends and future needs on the SIG's topics.
    \item Presentation (15 minutes): Each group will share their findings in a three-minute presentation to all attendees.
    \item Merge and discuss (20 minutes): Attendees will combine all findings on a single board, eliminating duplicates, labeling emerging themes, and identifying connections between themes.
    \item Final discussion (10 minutes): The organizers will lead a discussion focused on the consolidated board. The aim is to conclude the SIG with a clear map of current and future trends related to the SIG's topic.
    \item Lunch or dinner: Post-SIG, attendees are encouraged to join for a group lunch or dinner (at their own expense).    
\end{itemize}

\subsection*{Contacts}
Marios Constantinides from Nokia Bell Labs, Cambridge, UK, and Mohammad Tahaei from International Computer Science Institute, USA,  will be the first point of contact.
